# Supplementary material for: Machine Learning Domain Adaptation in Spin Models with Continuous Phase Transitions
Source: arXiv:2411.13027 source file (2025-11-18)
Supplement: Supplementary file 1 [file supplemental.pdf]

**Supplemental material** to the letter “Machine Learning Domain Adaptation in Spin Models with Continuous Phase Transitions” by Vladislav Chertnikov and Lev Shchur

**Spin and energy datasets.**— The dataset of spin configurations was generated by Markov chain Monte Carlo method with Metropolis single-spin update algorithm for the Ising and the Baxter-Wu models. Uncorrelated snapshots are generated on linear lattices of size  $L \in \{48, 72, 96, 144, 216\}$  in the temperature range  $[T_c - 0.4; T_c + 0.4]$  with  $N_{img} = 1500$  per temperature point  $T$ ,  $N_T \approx 110$ . The computer simulation is similar to what we used in our previous work, see reference [1] and the corresponding Supplementary Material.

The left part of Fig. 1 shows examples of spin configurations for the Ising and Baxter-Wu models, as well as conversions from the spin data set to the energy data sets for the Ising and Baxter-Wu models.

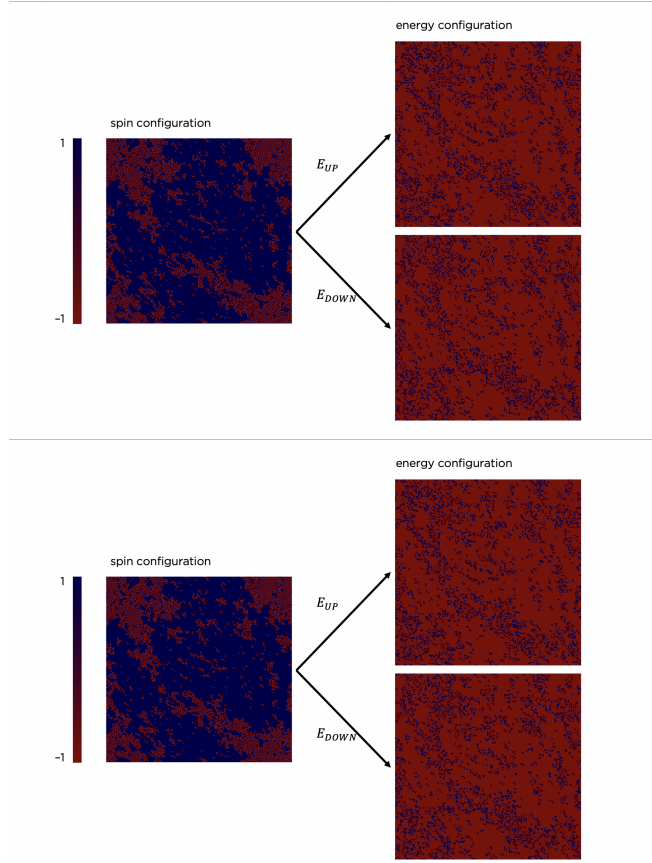

FIG. 1. Conversion of the spin dataset into energy datasets: the upper panel corresponds to the Ising model, the lower panel to the Baxter-Wu model,  $L = 216$ ,  $T = 2.2697$ .

**Machine learning on the spin dataset.** — The left panel of the fig. 2 shows estimates of the ferromagnetic (FM) phase probability calculated for Ising model using expr. (3) from Letter and fig. 3 the corresponding function  $V(T; L)$ , expr. (4) from Letter.

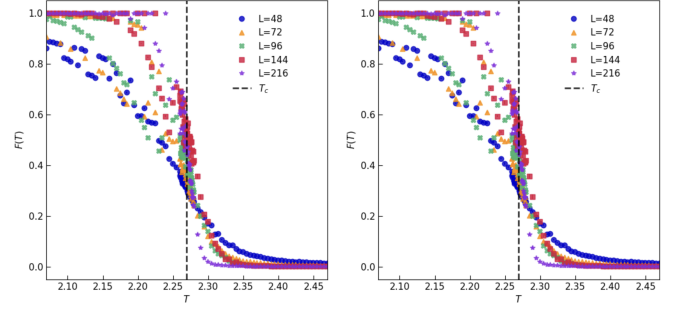

FIG. 2. The  $P(T; L)$  function estimated with CNN based on spin datasets. Left: training and testing using the Ising model – IS@IS. Right: training on the Baxter-Wu model and testing using the Ising model – IS@BW.

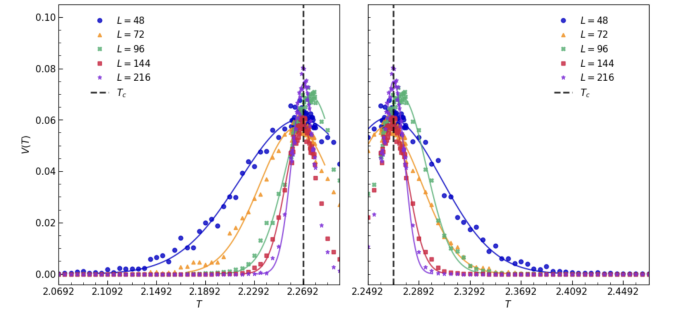

FIG. 3. The  $V(T; L)$  function estimated with CNN based on spin datasets. Training and testing using the Ising model.

The vertical dashed line corresponds to the exact value of the critical temperature  $T_c = 2.26918\dots$  separating FM and PM phases. The function plot  $P(T; L)$  for Ising model is similar to earlier publications and allows us to estimate the critical temperature using an approximation to the intersections of  $P(T; L)$  with the horizontal line at  $1/2$  [2].

The function  $V(T; L)$  allows us to estimate the correlation length exponent. Approximation of  $V(T; L)$  with the unnormalized Gaussian curves gives the width  $\sigma(L)$ . Alternatively, we may approximate separately the left and right wings of this function as shown in fig. 3, thus estimate  $\sigma^-(L)$  and  $\sigma^+(L)$ . This three functions used to estimates the inverse critical exponents  $1/\nu$  as

$$\sigma(L) \propto 1/L^{1/\nu} \quad (1)$$

$$\sigma^-(L) \propto 1/L^{1/\nu^-} \quad (2)$$

$$\sigma^+(L) \propto 1/L^{1/\nu^+} \quad (3)$$

and the corresponding values are shown in Table I.

The  $V(T)$  functions calculated for the Baxter-Wu model behave similarly to the Ising model, despite the fact that the Baxter-Wu spin configurations are defined on a triangular lattice. Table II summarises the  $1/\nu$  estimates for the Baxter-Wu model.

| IS@IS     | $1/\nu_\sigma$ | $1/\nu_{\sigma-}$ | $1/\nu_{\sigma+}$ |
|-----------|----------------|-------------------|-------------------|
| CNN       | 1.06(3)        | 1.11(5)           | 1.07(2)           |
| ResNet-10 | 1.25(3)        | 1.24(7)           | 1.25(3)           |

TABLE I. Estimates of the inverse correlation length exponent  $1/\nu$  for testing the Ising model on NN trained on the Ising model – IS@IS. Spin datasets used.

| BW@BW     | $1/\nu_\sigma$ | $1/\nu_{\sigma-}$ | $1/\nu_{\sigma+}$ |
|-----------|----------------|-------------------|-------------------|
| CNN       | 1.44(5)        | 1.54(6)           | 1.48(5)           |
| ResNet-10 | 1.47(5)        | 1.62(13)          | 1.46(4)           |

TABLE II. Estimates of the inverse correlation length exponent  $1/\nu$  for testing the Baxter-Wu model on NN trained on the Baxter-Wu model – BW@BW. Spin datasets used.

**Transfer learning with spin dataset.**— Fig. 4 and right panel of fig. 2 shows the case of knowledge transfer from the Baxter-Wu model to the Ising model – IS@BW. The function plot  $P(T; L)$  does not intersect other lattice sizes at the point  $1/2$ , as in the in-domain test (IS@IS), and the fluctuations of  $P(T, L)$  are observed in the ferromagnetic region, which makes the horizontal line approximation of the critical temperature less accurate. However, one can extract  $T_c$  from the peak position scaling of  $V(T; L)$  curve. The critical temperature  $T_c$  is more accurately determined by CNN rather than ResNet-10 if measured in absolute error units. The analytical solution of  $T_c$  lies within 2 standard deviations for both NNs. An estimate of critical exponent  $\nu$  cannot be extracted, although the NN output  $V(T; L)$  has a qualitatively similar Gaussian curve shape, the extracted values do not tend to a certain value.

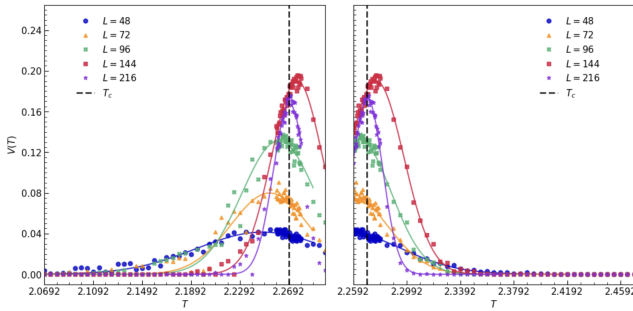

FIG. 4. CNN output  $V(T)$  function for spin configurations trained on Baxter-Wu model and tested on the Ising model – IS@BW.

As mentioned in the main text, the reverse cross-domain combination fails if NN is trained on the Ising model and tested on the Baxter-Wu model, BW@IS, on the space of spin configurations. The trained NNs have a predictive ability to separate images by phase in the Baxter-Wu model better than random guesses, when

measured by the roc-auc metrics – BW@IS. Still the function  $V(T)$  cannot be approximated to extract  $T_c$  and  $\nu$ .

**Energy dataset.**— The presence of two energy dataset matrices changes the structure of the input layers of NN architectures. In CNN and ResNet-10, the input convolutional layer now has two channels instead of one. The rest of the NN layers remain unchanged, as well as the training hyperparameters. Fig. 5 displays the NN output function  $V(T)$  for the Ising model CNN trained on the space of energy bonds – IS@IS.

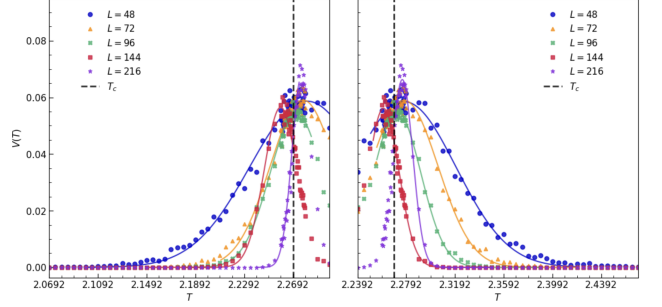

FIG. 5. CNN output  $V(T)$  function for energy bonds trained and tested on the Ising model – IS@IS.

For the Ising and the Baxter-Wu models, the critical temperature  $T_c$  is extracted to 4 decimal places using IS@IS and BW@BW procedures on energy datasets. The value of  $T_c$  lies within 1 standard deviation from the exact solution. The accuracy of extracting the critical exponent  $\nu$  from several parts of the  $V(T)$  curve for both combinations (IS@IS and BW@BW) is within 5 standard deviations in the Ising model, 1.5 in the Baxter-Wu model. The results are in agreement with the exact values of  $1/\nu$  in the corresponding universality classes. Encoding from spin configurations to the energy bond space did not improve the accuracy of the  $\nu$  exponent extraction. See the main text for the table content.

**Transfer learning with energy dataset.**— Fig. 6 shows a case of knowledge transfer from the Baxter-Wu model to the Ising model on the space of energy bonds – IS@BW. The opposite case, with BW@IS, is shown in the main text.

The critical temperature  $T_c$  is determined less accurately than in the domain test, within 3 standard deviations from the exact value for the Ising model and to 2 decimal places. The critical exponent  $\nu$  is within 4 standard deviations of the exact value for the Baxter-Wu model. The position of the maximum of the output variation function  $V(T; L)$  is non-systematic.

Knowledge transfer from the Ising model to the Baxter-Wu model - BW@IS. The critical temperature  $T_c$  is found to 4 decimal places within 1.5 standard deviations of the exact value. The critical exponent  $\nu$  is found within 2.5 standard deviations from the exact value for the Baxter-Wu model. We do not observe a regular be-

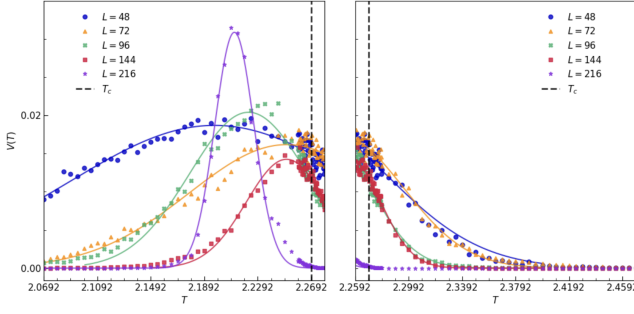

FIG. 6. CNN output  $V(T)$  function for energy bonds trained on Baxter-Wu model and tested on the Ising model – IS@BW.

haviour of the peak height  $V(T : L)$ , which behaves differently depending on the architecture - increasing with increasing  $L$  in CNN and decreasing in ResNet-10.

- 
- [1] V. Chertentkov, E. Burovski, and L. Shchur, Finite-size analysis in neural network classification of critical phenomena, Phys. Rev. E **108**, L031102 (2023).
  - [2] J. Carrasquilla and R.G. Melko, Machine learning phases of matter, Nat. Phys. **13**, 431 (2017).
